# Supplementary material for: Measurement of Coherent Elastic Neutrino-Nucleus Scattering from reactor antineutrinos
Source: arXiv:2202.09672 ancillary file (2022-11-19)
Supplement: Supplementary file 1 [file READ_ME.pdf]

# NCC-1701 data release

October 2021

**Description of attached data files:** the present release consists of three data files: `data.txt`, `iron_filter.txt` and `photo_neutron.txt`. The first file corresponds to the data displayed in Fig. 1 of the publication accompanying this release. The file format is as follows. First column: energy in keV (bin center). Second column: counts/10 eV·3 kg·day for 96.4 days of Rx-ON operation. Third column: error bar (combination of statistical and signal acceptance uncertainties -see Fig. 1 below-). Fourth column: counts/10 eV·3 kg·day for 25 days of Rx-OFF operation. Fifth column: error bars, as before. The rest of the data files are discussed further below.

**Energy resolution:** the calculated CE $\nu$ NS differential signal rate needs to be smeared by the intrinsic energy resolution of the detector. Following [1, 2] this resolution is described by an energy-dependent Gaussian width  $\sigma^2 = \sigma_n^2 + E\eta F$ . The first term  $\sigma_n$  represents the intrinsic electronic noise of the detector, on average 68.5 eV during the 96.4 days of Rx-ON data and 65.25 eV during the 25 days of Rx-OFF operation. The second term describes the dispersion in the number of information carriers (electron-hole pairs):  $E$  is the ionization energy in eV,  $\eta = 2.96$  eV is the average energy of electron-hole formation in Ge, and  $F$  is the Fano factor. Fits to the K- and L-shell EC peaks yield values of  $F \sim 0.10$ - $0.11$ , in good agreement with [3]. A small energy-dependence of  $F$  as described in [3] can be applied to the calculation of the CE $\nu$ NS signal, but its effect is seen to be tiny.

**Background from M-shell electron capture (EC) in  $^{71}\text{Ge}$ :** the contamination from this process, which appears next to threshold in the CE $\nu$ NS ROI can be treated during spectral fits as follows. First, the L-shell EC peak at a nominal energy of 1.297 keV, corresponding to the electron binding energy of the gallium daughter [4], can be described by a Gaussian PDF with three free parameters, an amplitude  $a$ , a centroid  $b$ , and standard deviation

$\sigma$  (once fitted, a Fano factor can be extracted from  $\sigma$  as above). The area (number of counts) under this peak will then be given by:

$$A_L = \int_{-\infty}^{\infty} a e^{-(E-b)^2/(2\sigma^2)} dE = a|\sigma|\sqrt{2\pi}$$

The ratio  $A_M/A_L$  has been experimentally determined to be  $0.16 \pm 0.03$  [5], in good agreement with a theoretical expectation of 0.17 [6]. We can then express the amplitude  $a'$  of the M-shell EC peak as  $a' = 0.16 a \frac{\sigma}{\sigma'}$ , where  $\sigma'$  is its standard deviation. The centroid for this peak  $b'$  is below detector threshold and as such it cannot be reliably extracted from a fit to the data. Instead, its nominal value of 0.158 keV [4, 5] must be used. Similarly, following the discussion above,  $\sigma'$  is to an excellent approximation just equal to the electronic noise  $\sigma_n$ . These considerations fully define the three parameters  $a', b', \sigma'$  describing the M-shell EC peak, with  $a'$  nevertheless being a function of the L-shell peak parameters. The present state of knowledge about  $A_M/A_L$  is accounted for during MCMC analysis by allowing the factor 0.16 in the expression for  $a'$  to float over its  $\pm 0.03$  uncertainty, constrained by a Gaussian prior of that width.

**Contribution from L<sub>2</sub>-shell EC:** the discussion above refers to EC from the dominant L<sub>1</sub>-shell. Electron capture from the L<sub>2</sub>-shell is possible, resulting in an additional peak at  $E_{L_2} = 1.142$  keV [4]. However, this happens with a small probability: for  $Z = 32$ , the ratio  $A_{L_2}/A_{L_1}$  is calculated to be  $\sim 0.008$ , with a negligible  $A_{L_3}/A_{L_1}$  [7, 8, 9]. While this was not remarked in [5], an excess above background at the expected position of the L<sub>2</sub> peak is visible and resolved from L<sub>1</sub> in Fig. 3 of that publication. This confirms the need to account for this spectral component, but provides no experimental value for  $A_{L_2}/A_{L_1}$ . We treat L<sub>2</sub>-shell EC similarly to the discussion above: to an excellent approximation, the width of L<sub>2</sub> and L<sub>1</sub> peaks is the same, and  $E_{L_2} = 1.142$  keV can be imposed as the L<sub>2</sub> peak centroid. The theoretical  $A_{L_2}/A_{L_1} = 0.008$  ratio is then the same as the ratio between the L<sub>2</sub> and L<sub>1</sub> peak amplitudes. This accounts for this small spectral component without the need to introduce additional free parameters.

**Quenching factor models:** the publication associated to this data release discusses two quenching factor models originally presented in Sec. VI of [10]. The first combines a low-energy linear fit to iron filter measurements of the quenching factor (QF) for germanium, with higher-energy Lindhard theory predictions for the same. The file `iron_filter.txt` contains the four iron filter datapoints from Fig. 9 in [10]. First column is  $E(\text{keV}_{nr})$ , 2nd is QF(%),

3rd is the horizontal error, 4th top vertical error, 5th bottom vertical error. The file `photo_neutron.txt` contains information for the photo-neutron QF model shown in the same figure. First, third and fifth columns are energies in  $\text{keV}_{nr}$ . The 2nd column is the best-fit QF ( $Y=0.86$  [10]) in %, fourth is the  $+2\sigma$  boundary ( $Y=0.90$ ), and sixth is the  $-2\sigma$  boundary ( $Y=0.82$ ). Small fluctuations in these fits were smoothed out in Fig. 9 of [10]. These files can be used to create QF PDFs, which can then be adopted for CE $\nu$ NS signal predictions. Our own fits in this respect are shown in Fig. 1 below.

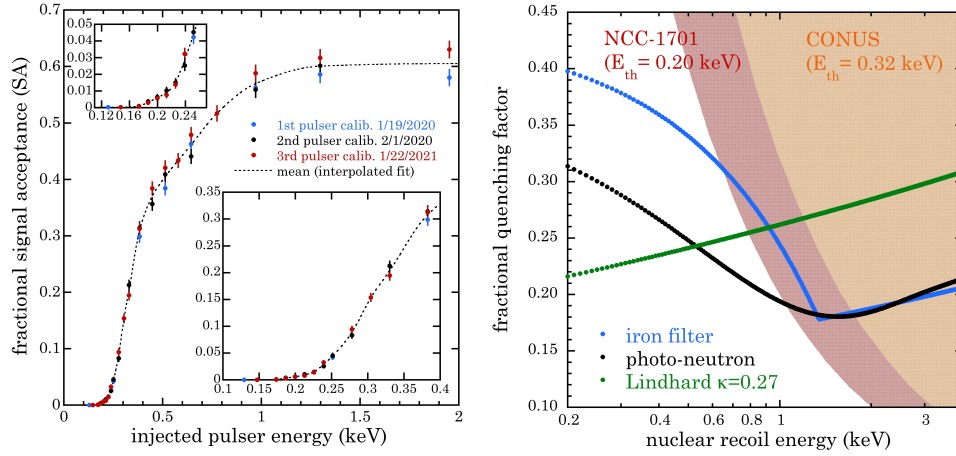

Figure 1: *Left:* Signal acceptance (SA) following all data cuts, determined using a programmable pulser mimicking the rise-time of bulk events in the PPC. The effect of progressive cuts on this SA is described in [11]. All measurements collected during three separate calibrations are shown. Error bars are statistical. Insets highlight low-energy regions. Three methods of interpolation were tested to fit the mean of these measurements [12]. Their differences are  $< 1\%$ , except for a divergence of order 2% above 1.5 keV due to the scarcity of datapoints in that region. The standard error of the mean is fitted to provide a smoothly-varying uncertainty in the SA (8.6% at threshold, going through a minimum of 1.3%, and back up to 4.4% at 2 keV). *Right:* Two QF models based on data from [10], together with a  $\kappa=0.27$  Lindhard model excluded by CONUS [13]. Lower values of  $\kappa$  remain allowed ( $\kappa$  approximately corresponds to the Lindhard fractional QF value at 1 keV, with same energy dependence as in the figure elsewhere.  $\kappa = 0.157$  is the nominal value for Ge [10]). Colored regions indicate the approximate reach in QF sensitivity for each experiment as a result of their different thresholds  $E_{th}$ , when the effect of energy resolution is neglected.

**Including CONUS constraints:** we have considered a number of ways to account for recent CONUS limits on germanium QF models [13] in our analysis. The differences in energy resolution between detectors and the variety of possible QF models make this less than straightforward. Aiming to reduce the introduction of arbitrary choices when applying these constraints, we have adopted the following approach: the main deliverable from [13] is that Lindhard QF models with free parameter  $\kappa > 0.27$  (Fig. 1 here) are excluded by CONUS data. The limiting model ( $\kappa = 0.27$ ) would generate an integrated 6.83 CE $\nu$ NS counts above 320 eV in our detector during its 96.4 day Rx-ON exposure, accounting for the effect of energy resolution. This energy is the average detector threshold used by CONUS in their analysis, computed weighting each detector by its contribution to total exposure [13]. When allowing CE $\nu$ NS signal models to follow a free exponential form (see Fig. 4 in the publication accompanying this release) we impose a Gaussian prior of width 6.83 counts on the integrated count rate above 320 eV that these models predict. This has a limited impact over the parameter space shown in that figure, but it penalizes any unphysical solutions beyond, now excluded by CONUS.

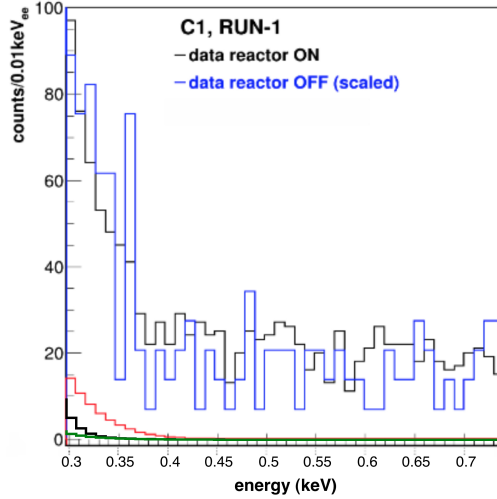

Figure 2: (adapted from [13]) Comparison between CONUS Rx-ON and Rx-OFF spectra and several CE $\nu$ NS predictions: signal at the 90% C.L. exclusion limit derived from CONUS data (red [13]), Fe-filter QF model + Kopeikin flux (black), Y/Be QF model + Kopeikin flux (green).



Fig. 2 above shows the expected  $\text{CE}\nu\text{NS}$  signal for Fe-filter and Y/Be QF models and the Kopeikin neutrino spectrum discussed in the publication accompanying this release. The calculation is done for a Brokdorf reactor flux of  $2.3 \times 10^{13} \bar{\nu}_e/\text{cm}^2\text{s}$  and a 96.7 kg-day (detector C1, run-I) CONUS exposure [13], using a C1 detector resolution of 69 eV FWHM [14]. We notice a tendency for our integrated rate calculations to surpass those by CONUS (Fig. 4 in [13]) by a factor 30%-50%, something not observed in comparisons with other authors. Even with that, these QF models -favored by our work- are not in tension with present CONUS data. Fig. 1 in this release illustrates the comparative reach of CONUS and NCC-1701 in QF parameter space.

**MCMC corner plots:** the four following pages display MCMC corner plots resulting from the analysis of Rx-ON and Rx-OFF datasets. These are provided for both alternative ( $H_1$ ) and null ( $H_0$ ) hypotheses. These plots correspond to the first step in the statistical analysis described in the publication accompanying this release, where the  $\text{CE}\nu\text{NS}$  signal is approximated by an exponential. This approximation is introduced for the purpose of identifying the quenching factor models most favored by the data. A second step in the analysis is used to quantify the rejection of  $H_0$  in favor of  $H_1$  for several identified cases of interest, via their Bayes factors, removing approximations and free parameters from the Standard Model  $\text{CE}\nu\text{NS}$  predictions.

The parameters shown in these plots are as follows (the span of their uniformly sampled parameter space and its units are provided between parentheses): **Bckgr\_tau** ([0.0,2.0]  $\text{keV}_{ee}$ ) is the decay constant for the exponential component of the epithermal neutron background model, **Bckgr\_amp** ([0,150] counts / 10 eV 3 kg day) its amplitude at 0.2  $\text{keV}_{ee}$ , and **Const** ([0,25] counts / 10 eV 3 kg day) the constant term in the epithermal model. **CEvNS\_amp** ([0,40] counts / 10 eV 3 kg day) and **CEvNS\_tau** ([0.00,0.08]  $\text{keV}_{ee}$ ) correspond to  $A_{0.2}$  and  $\xi$  in Fig. 4 of the accompanying publication, respectively. **L1\_amp** ([70,250] counts / 10 eV 3 kg day), **L1\_mean** ([1.2,1.4]  $\text{keV}_{ee}$ ) and **L1\_sig** ([0.04,0.10]  $\text{keV}_{ee}$ ) are the  $L_1$  EC peak parameters  $a$ ,  $b$ ,  $\sigma$  discussed earlier in this data release, respectively, and **M\_ratio** ([0.0,0.3]) is the adimensional numerical factor in the expression for  $a'$  also described above. This last parameter is constrained by a Gaussian prior mentioned there.

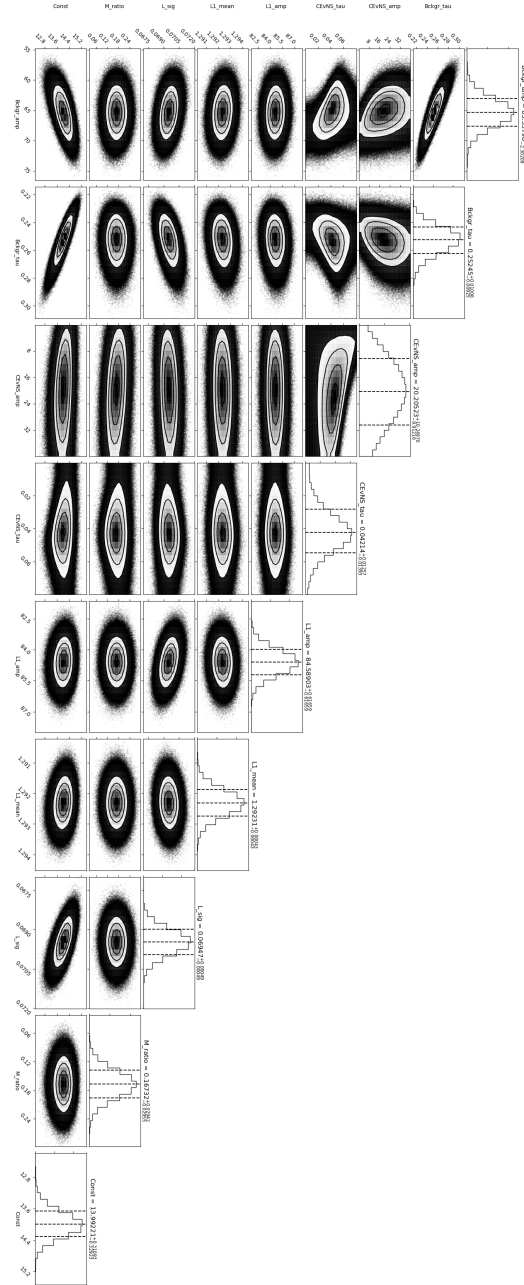

Figure 3: MCMC corner plot for Rx-ON, alternative hypothesis.

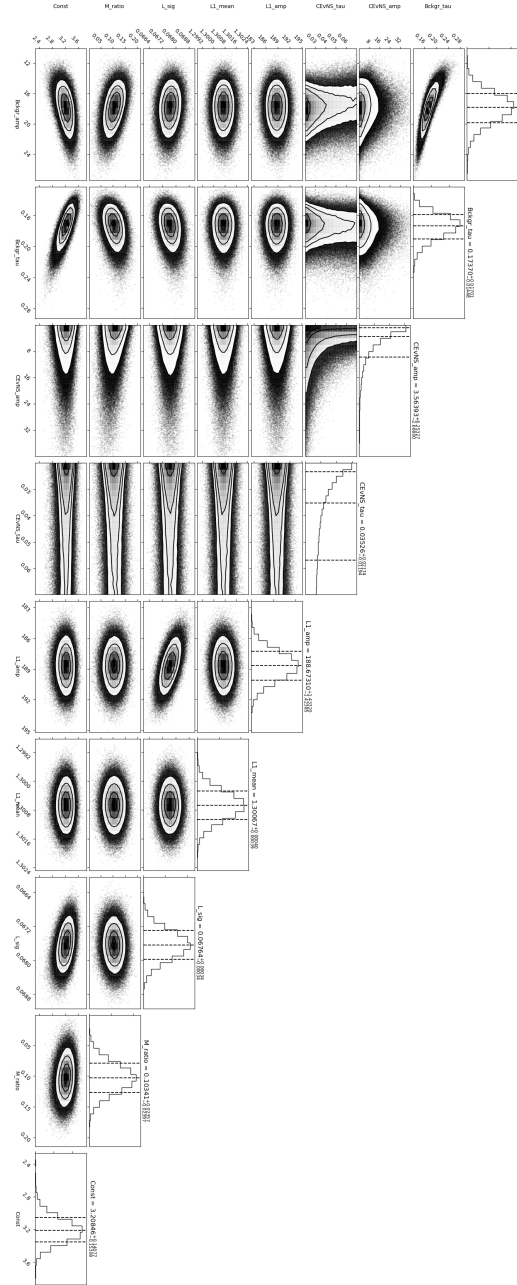

Figure 4: MCMC corner plot for Rx-OFF, alternative hypothesis.

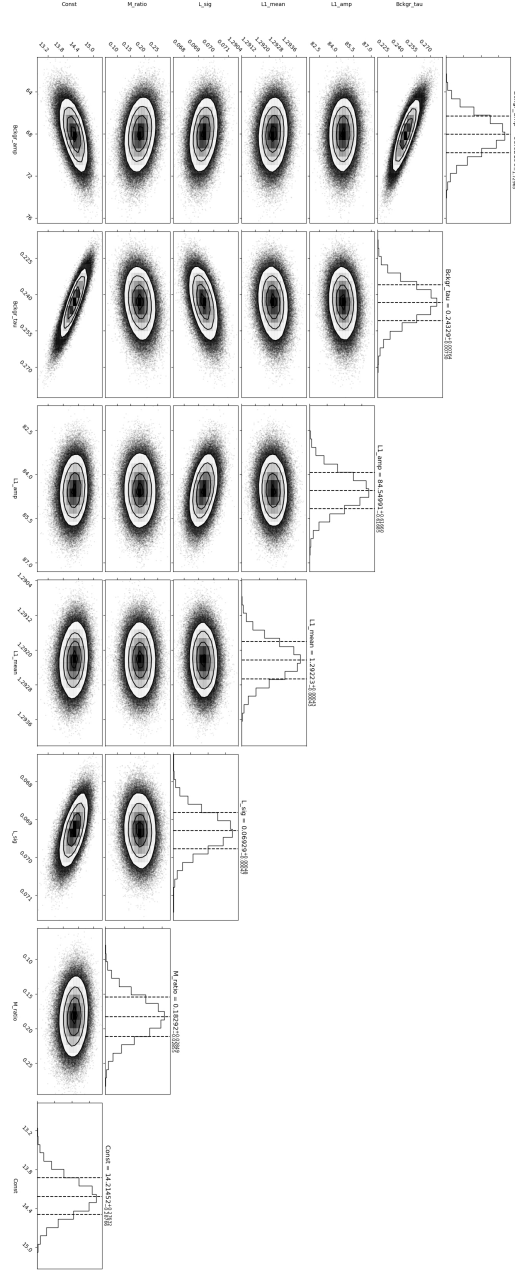

Figure 5: MCMC corner plot for Rx-ON, null hypothesis.

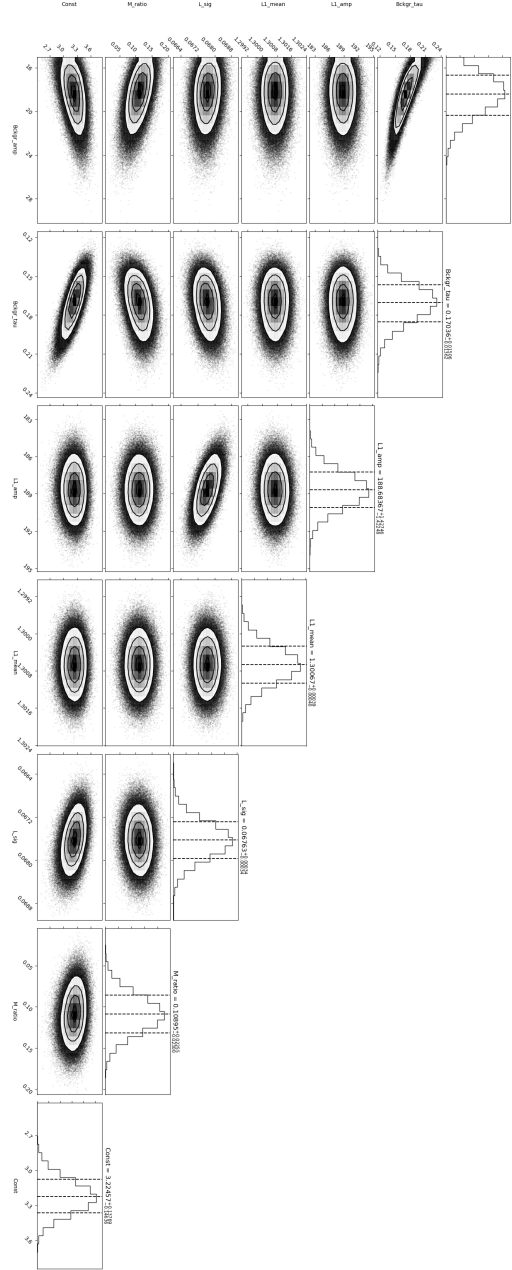

Figure 6: MCMC corner plot for Rx-OFF, null hypothesis.

**Additional comments on statistical analysis:** a parametrization of the  $\text{CE}\nu\text{NS}$  signal as an exponential with free amplitude and free decay constant is useful during a first step of statistical analysis aiming to determine the quenching factor model(s) most favored by the data. This is the subject of the discussion around Fig. 4 in the Letter accompanying this data release. However, this (rough) approximation introduces two unnecessary arbitrary parameters in the description of the  $\text{CE}\nu\text{NS}$  signal: once a choice of QF and neutrino energy spectrum has been adopted, the Standard Model univocally defines a  $\text{CE}\nu\text{NS}$  signal devoid of free parameters.

In a second step of the analysis, the null hypothesis  $H_0$  (background model only) is compared to several alternative hypotheses  $H_1$  which include, in addition to the background, exact Standard Model  $\text{CE}\nu\text{NS}$  predictions calculated for six combinations of QF and neutrino spectrum found to be of most interest. When doing so,  $H_0$  and  $H_1$  models contain the same number of free parameters, those associated to the description of the background. This limits the choice of statistical estimators available for model selection. A widely-used likelihood ratio test (the default frequentist approach to hypothesis testing) requires  $H_0$  and  $H_1$  to be nested [15, 16], clearly not the present case. Most importantly, the test statistic in this method (the change in deviance  $\Delta D$  between the best-fit  $H_0$  and  $H_1$ ) is expected to follow a chi-square distribution with degrees of freedom equal to the difference in model dimensionality  $k$ , restricting the applicability of the likelihood ratio to instances where null and alternative hypotheses differ by at least one free parameter ( $k \geq 1$ ) [15].

A Bayes factor test like that used in this Letter, while also commonplace, has the advantage of not being affected by these restrictions in applicability. Another popular method able to compare the quality of statistical models and to rank them, similarly free of these limitations, is the relative likelihood [17, 16]. It is closely related to the likelihood ratio and based on the so-called Akaike information criterion ( $AIC$  [18]), derived from information theory [17]. In this context, the relative likelihood of the alternative hypothesis with respect to the null hypothesis is quantified by  $\exp(\frac{AIC(H_0) - AIC(H_1)}{2})$ . In the limit where  $k = 0$ , the present situation, this expression reduces to  $\exp(\frac{\Delta D}{2})$ , which is then also equivalent to the ratio between the maximum value of the likelihood function for  $H_1$  and that for  $H_0$  [16, 19]. Not surpris-

ingly, the preference obtained for  $H_1$  over  $H_0$  using this additional approach to model selection is very similar to that derived via the Bayes factor: for Rx-ON, the Fef QF model yields a relative likelihood of 28.2 (MHVE) and 27.3 (Kopeikin). For the YBe QF this becomes 11.5 (MHVE) or 8.7 (Kopeikin). For a Lindhard QF the values are 3.3 and 2.6, respectively.

As per the discussion above, a direct comparison of the difference in  $AIC$  values between two competing hypotheses and the  $p$ -value returned by their likelihood ratio test can only be established for  $k \geq 1$ . However, their observed correlation points to a  $p$ -value  $\ll 0.005$  in the  $k \rightarrow 0$  limit [16, 19] for the most-favored  $H_1$  options assessed here (Fef-MHVE and Fef-Kopeikin, for which  $\Delta D$  is 6.7 and 6.6, respectively). The evolution of the  $p$ -value with decreasing  $k$  at  $\Delta D = 6.7$  indicates that  $9.9 \times 10^{-4} < p < 1.2 \times 10^{-3}$  in the limit  $k \rightarrow 0$ . This is in the realm of  $p$ -values typically interpreted as “convincing evidence” for the alternative hypothesis (presence of  $CE\nu NS$ ), and well beyond the conventional “suggestive evidence” range ( $0.05 \lesssim p \lesssim 0.1$ ) [16, 20].

As a final note in this section, Fig. 7 below shows null hypothesis best-fits to the 37 day and 20 day Rx-ON datasets presented in an earlier publication [11]. Those correspond to periods of considerably-higher epithermal neutron interaction rate than presently achieved, by factors of  $\sim \times 6$  and  $\sim \times 2$ , respectively. The background model adopted in this Letter is further validated by the excellent fit observed for these background-dominated datasets.

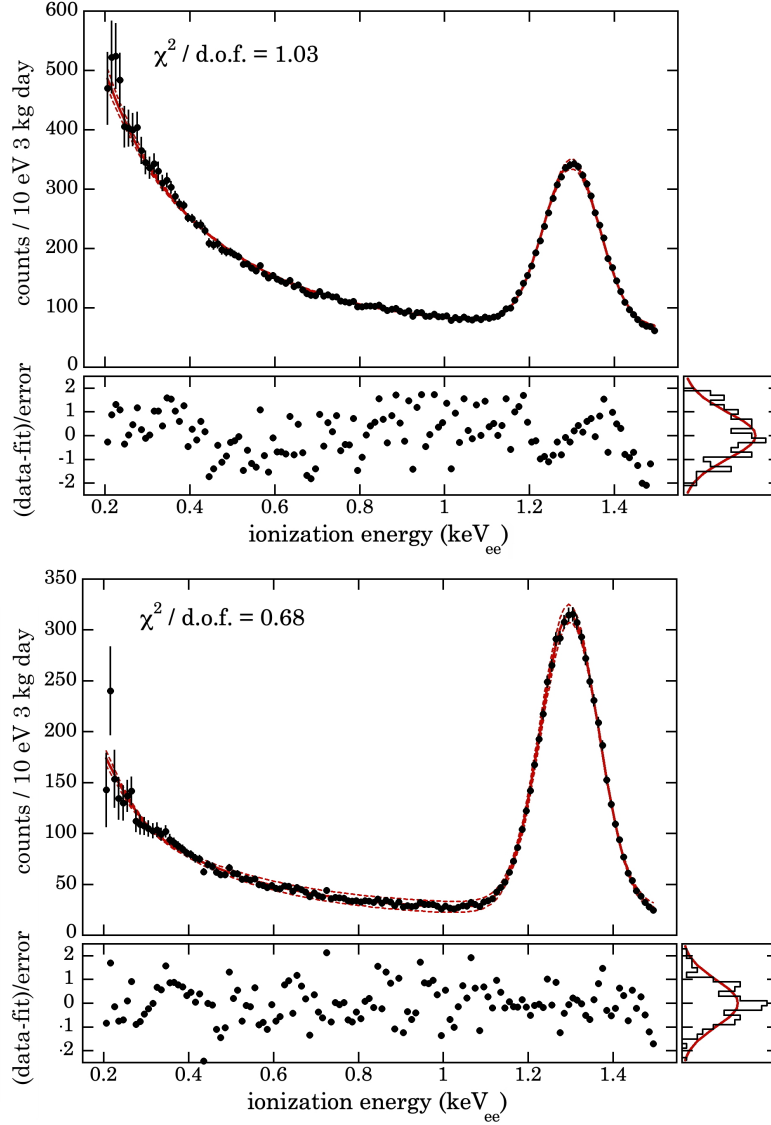

Figure 7: MCMC fits of the null hypothesis to neutron-dominated 37 day (top) and 20 day (bottom) Rx-ON datasets from [11] (see text). For consistency, these data have been re-analyzed with final cuts and the cumulative signal acceptance discussed above. A solid red line indicates the best-fit background model, dashed lines its  $\pm 1\sigma$  posterior spread. Reduced chi-square values are shown. A bottom panel displays standardized residuals. Side panels show their distribution (histogram) and expected Gaussian spread (line).



## References

- [1] C. E. Aalseth et al. “Experimental Constraints on a Dark Matter Origin for the DAMA Annual Modulation Effect”. In: *Phys. Rev. Lett.* 101 (2008), p. 251301.
- [2] C. E. Aalseth et al. “Erratum: Experimental Constraints on a Dark Matter Origin for the DAMA Annual Modulation Effect”. In: *Phys. Rev. Lett.* 102 (2009), p. 109903.
- [3] B.G. Lowe. “Measurements of Fano factors in silicon and germanium in the low-energy X-ray region”. In: *Nucl. Instr. Meth. A* 399 (1997), pp. 354–364.
- [4] Richard B. Firestone and Virginia S. Shirley. *Table of Isotopes*. New York: Wiley, 1996.
- [5] R. Agnese et al. “New Results from the Search for Low-Mass Weakly Interacting Massive Particles with the CDMS Low Ionization Threshold Experiment”. In: *Phys. Rev. Lett.* 116 (2016), p. 071301.
- [6] E. Schönfeld. “Calculation of fractional electron capture probabilities”. In: *Applied Radiation and Isotopes* 49 (1998), pp. 1353–1357.
- [7] E.J. Konopinski and M.E. Rose. “The theory of nuclear  $\beta$ -decay”. In: *Alpha-, Beta- and Gamma-Ray Spectroscopy*. Ed. by K. Siegbahn. Amsterdam: North-Holland, 1965.
- [8] X. Mougeot. “Towards high-precision calculation of electron capture decays”. In: *Applied Radiation and Isotopes* 154 (2019), p. 108884.
- [9] X. Mougeot, private communication.
- [10] J. I. Collar, A. R. L. Kavner, and C. M. Lewis. “Germanium response to sub-keV nuclear recoils: A multipronged experimental characterization”. In: *Phys. Rev. D* 103 (2021), p. 122003.
- [11] J. Colaresi et al. “First results from a search for coherent elastic neutrino-nucleus scattering at a reactor site”. In: *Phys. Rev. D* 104 (2021), p. 072003.
- [12] MATLAB implementation of Piecewise Cubic Hermite Interpolating Polynomial (PCHIP), modified Akima piecewise cubic Hermite interpolation, and cubic spline methods.

- [13] H. Bonet et al. “Constraints on Elastic Neutrino Nucleus Scattering in the Fully Coherent Regime from the CONUS Experiment”. In: *Phys. Rev. Lett.* 126 (2021), p. 041804.
- [14] Janina Dorin Hakenmüller. PhD thesis. Heidelberg University, 2020.
- [15] S. S. Wilks. “The Large-Sample Distribution of the Likelihood Ratio for Testing Composite Hypotheses”. In: *The Annals of Mathematical Statistics* 9.1 (1938), pp. 60–62. URL: <https://doi.org/10.1214/aoms/1177732360>.
- [16] Paul A. Murtaugh. “In defense of P values”. In: *Ecology* 95.3 (2014), pp. 611–617. eprint: <https://esajournals.onlinelibrary.wiley.com/doi/pdf/10.1890/13-0590.1>.
- [17] K.P. Burnham and D.R. Anderson. *Model Selection and Multimodel Inference: A Practical Information-Theoretic Approach*. Springer New York, 2003. ISBN: 9780387953649.
- [18] H. Akaike. “A New Look at the Statistical Model Identification”. In: *IEEE Transactions on Automatic Control* 19 (Jan. 1974), pp. 716–723.
- [19] Roger Mundry. “Issues in information theory-based statistical inference—a commentary from a frequentist’s perspective”. In: *Behavioral Ecology and Sociobiology* 65 (2010), pp. 57–68.
- [20] Fred L. Ramsey and Daniel W. Schafer. *The Statistical Sleuth : A Course in Methods of Data Analysis*. Brooks/Cole, Cengage Learning, 2002. ISBN: 9781133490678.
